# Supplementary material for: Helping Blind People Grasp: Enhancing a Tactile Bracelet with an Automated Hand Navigation System
Source: arXiv:2504.16502 source file (2025-04-23)
Supplement: Supplementary file 1 [file suplementary_material.pdf]

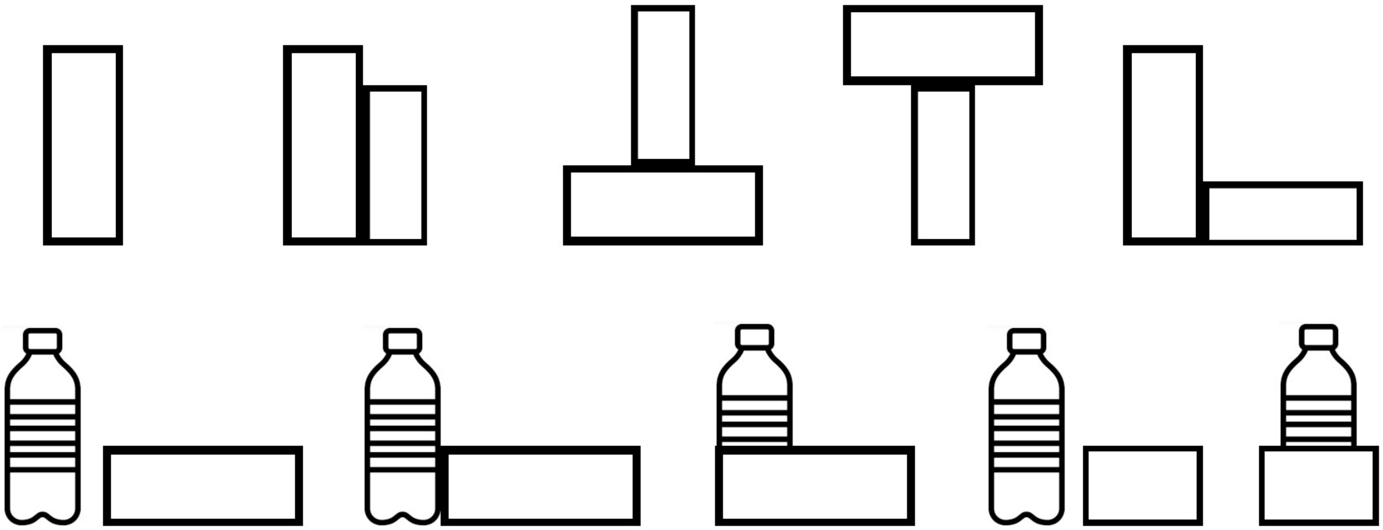

Figure S1: All possible placements of the boxes to create an obstacle in the depth navigation task as seen from the participants' perspective. In each case, the target object was placed on the left side of the obstacle and the hand was placed on the right side of the obstacle. In the upper row, obstacles preventing the horizontal movement of the hand to the target are presented. In the lower row, the relative positions of the obstacle and target object for standard navigation are presented.

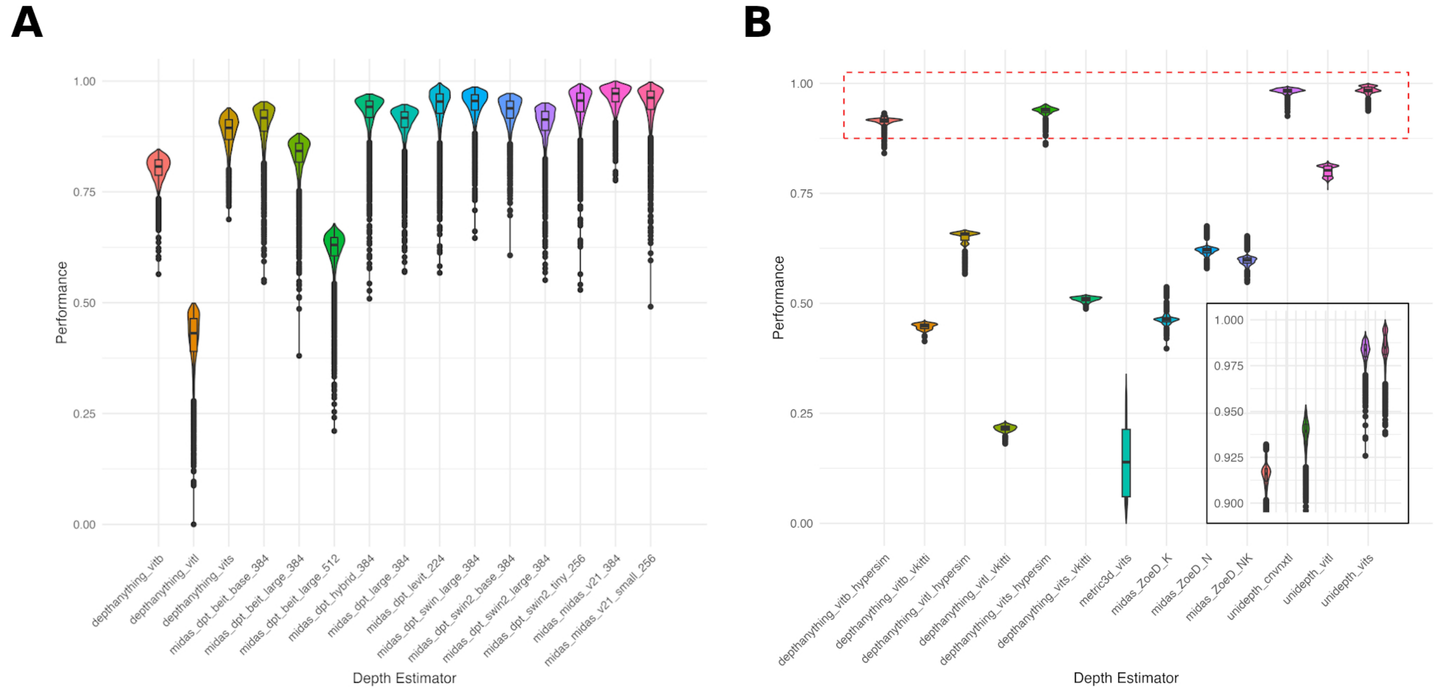


Figure S2: A) Violin plot of mean normalized performance score per relative depth estimator. Each point in the plot represents the depth estimate for one object. The performance score is then the weighted and variance-penalized linear combination of speed and accuracy of the respective estimator, averaged across all data points, and normalized afterwards. B) Violin plot of mean normalized performance score per metric depth estimator. A zoom-in on the top 10% can be found in the lower right corner.

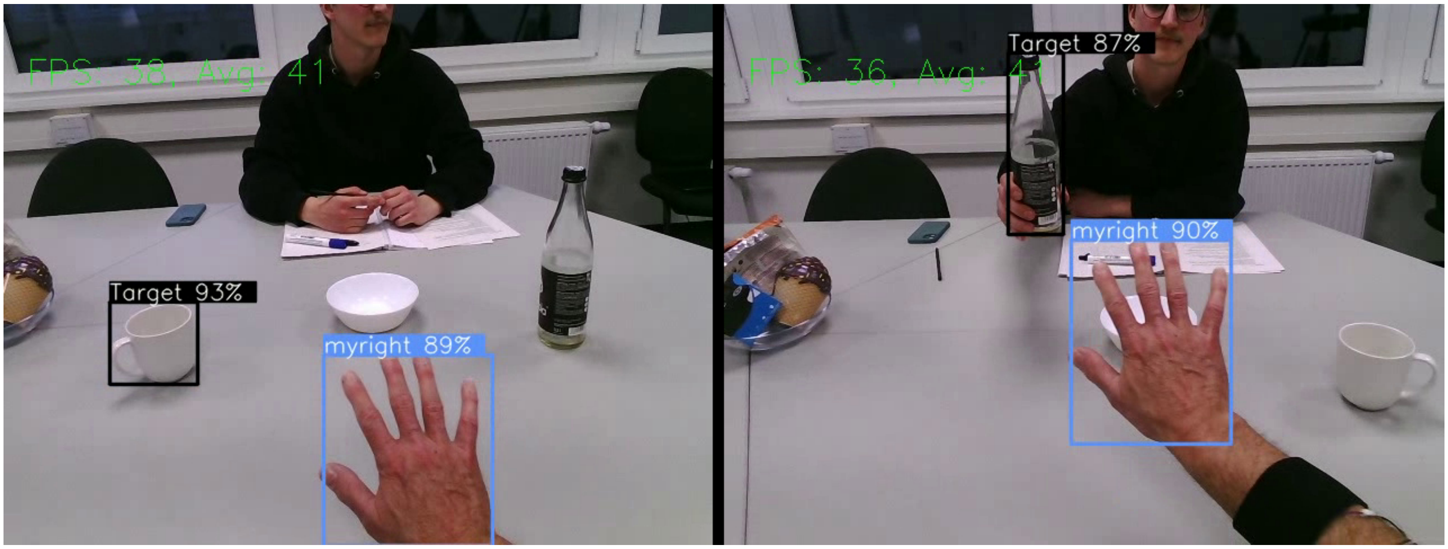


Figure S3: Output of the system in the grasping trial (on the left) and during interaction (on the right). The hands of the experimenter, serving as distractors, are not detected, enabling the user's hand to successfully navigate to the target object.

Table S1: Topics and closed questions with the score aggregated for each topic across participants.

| Topic | Question 1 | Question 2 | Median | Mean | SD |
|---|---|---|---|---|---|
| discomfort | The vibrations from the bracelet unpleasantly numbed my skin. | The bracelet felt uncomfortable on my wrist. | 1.0 | 1.25 | 0.46 |
| guidance | The vibration direction commands were giving a consistent path. | I could feel irrational jumping of vibration directions during the grasping guidance. | 4.0 | 4.13 | 0.99 |
| interpretability | I could easily differentiate vibration direction commands throughout the grasping tasks. | It was difficult for me to interpret the vibration direction commands from the tactile bracelet. | 4.0 | 3.63 | 0.74 |
| reliability | I felt like I could depend on the bracelet to not hit any objects in my grasping path. | I rather relied on my intuition than on the bracelet for navigating my hand. | 5.0 | 4.75 | 0.46 |
| responsiveness | The tactile bracelet was satisfyingly responsive during the guidance of my hand. | I had to adjust my hand movements because of lagging tactile feedback. | 4.0 | 3.63 | 1.19 |
| engagement | It was fun using the tactile bracelet. | I got frustrated using the tactile bracelet. | 4.0 | 4.38 | 0.52 |
| simplicity | The grasping tasks were manageable with the tactile bracelet. | I felt like I could not perform the grasping tasks well using the tactile bracelet. | 4.0 | 3.63 | 1.19 |
| training | The training phase was sufficient to get comfortable with using the tactile bracelet. | The training did not help me enough to manage the grasping tasks confidently. | 5.0 | 4.38 | 1.06 |
| vibrations | I found the vibration intensity to be consistent. | The felt vibration intensity varied strongly. | 4.5 | 4.50 | 0.54 |

Table S2: Details of the training runs of the object detectors. Runs labeled as COCO indicate networks for objects, labeled as EgoHands for hands detection.

| Run | Model | Resolution | Batch Size | Epochs | Precision | Recall | mAP 50 | mAP 50-95 |
|---|---|---|---|---|---|---|---|---|
| COCO baseline | 5s | 640 | 16 | 100 | 0.70 | 0.58 | 0.62 | 0.42 |
| COCO1 | 5s | 640 | 16 | 300 | 0.69 | 0.57 | 0.60 | 0.41 |
| COCO2 | 5s | 640 | 32 | 300 | 0.69 | 0.57 | 0.60 | 0.41 |
| COCO3 | 5s 6 | 1280 | 16 | 130 | 0.72 | 0.62 | 0.65 | 0.46 |
| COCO4 | 5m | 640 | 16 | 259 | 0.73 | 0.61 | 0.64 | 0.46 |
| COCO5 | 5m | 640 | 32 | 251 | 0.74 | 0.60 | 0.64 | 0.46 |
| COCO6 | 5m 6 | 1280 | 32 | 130 | 0.74 | 0.65 | 0.69 | 0.51 |
| COCO7 | 5l | 640 | 16 | 181 | 0.74 | 0.64 | 0.68 | 0.49 |
| COCO8 | 5l | 640 | 32 | 155 | 0.74 | 0.64 | 0.68 | 0.49 |
| COCO9 | 5l 6 | 1280 | 32 | 130 | 0.76 | 0.65 | 0.70 | 0.52 |
| COCO10 | 5xl | 640 | 16 | 138 | 0.74 | 0.65 | 0.69 | 0.50 |
| COCO11 | 5xl | 640 | 32 | 151 | 0.73 | 0.65 | 0.69 | 0.50 |
| COCO12 | 5xl 6 | 1280 | 32 | 100 | NA | NA | NA | NA |
| EgoHands1 | 5s | 640 | 32 | 240 | 0.98 | 0.97 | 0.99 | 0.81 |
| EgoHands2 (augmented) | 5s | 640 | 32 | 300 | 0.98 | 0.97 | 0.98 | 0.81 |
